# Supplementary material for: How Can LLM Guide RL? A Value-Based Approach
Source: arXiv:2402.16181 source file (2024-02-25)
Supplement: Supplementary file 1 [file appendix.tex]

\section{Proofs}

\subsection{Proof of Theorem \ref{thm_vanilla_com}}
\begin{proof}
%From Assumption \ref{assump_topk}, we know that $\mathbb{P}_{\text{LLM}}(a_t | s_t^*) \leq 1 / k$ for any $t\in[1,T]$ and $a_t\notin \mathcal{A}_{\text{topk}}$. This can be shown by contradiction. Specifically, if there exists $\mathbb{P}_{\text{LLM}}(a_t | s_t^*) > 1 / k$ for some $a_t\notin \mathcal{A}_{\text{topk}}$, then $\mathbb{P}_{\text{LLM}}(a'_t | s_t^*) > 1 / k$ for all $a'_t\in \mathcal{A}_{\text{topk}}$. In this case, the sum of probabilities is greater than $1$, which is a contradiction.

%Therefore, for any $t\in[1,T]$, it holds that 
%\$
%\mathbb{P}_{\text{LLM}}(a_t^* | s_t^*, g) \geq 1-\frac{1}{k}\cdot\bigl(|\mathcal{A}|-k\bigr)=2-\frac{|\mathcal{A}|}{k}.
%\$

We denote $\varsigma = \min_{s_t\in\mathcal{S}}\mathbb{P}_{\text{LLM}}(\pi_t^*(s_t, g)|s_t, g) > 0$. Then we obtain that with probability at least $1/2$, the value of the LLM policy satisfies 
\#\label{eq_app_v_vanilla}
V_1^{\mathbb{P}_{\text{LLM}}}(s_1, g) = \prod_{t=1}^T \mathbb{P}_{\text{LLM}}(a_t^* | s_t^*, g)\cdot 1 > \varsigma^T.
\#

Denote by $\Tilde{V}_1^{\mathbb{P}_{\text{LLM}}}(s_1, g)$ the average cumulative reward in $\varsigma^{2T}\log(1/\delta)/2$ episodes. Then we have from the Hoeffding's inequality that
\$
\mathbb{P}\Biggl(\Tilde{V}_1^{\mathbb{P}_{\text{LLM}}}(s_1, g) - V_1^{\mathbb{P}_{\text{LLM}}}(s_1, g) > -\biggl(\frac{1}{\varsigma}\biggr)^T\Biggr) \geq 1 - \exp\Bigl(-2\cdot \frac{\log(1/\delta)}{2}\varsigma^{2T}\cdot\varsigma^{-2T}\Bigr) = 1-\delta.
\$

Combining with the result in \eqref{eq_app_v_vanilla}, it holds with probability at least $1-\delta$ that $\Tilde{V}_1^{\mathbb{P}_{\text{LLM}}}(s_1, g) > 0$, indicating that the vanilla LLM-based planning is optimal since the agent receives a $1$ reward only when reaching the goal in the sparse-reward setting.

The result of the sample number $T\varsigma^{2T}\log(1/\delta)/2$ is then obtained by noting that each episode contains $T$ samples.

For the worst-case sample complexity bound, we refer to the proof of Theorem 2.1 in \cite{laidlaw2023bridging}.
\end{proof}

\subsection{Proof of Proposition \ref{prop_rew_shaping}}
\begin{proof}
The posterior distribution over the actions when conditioning on $\mathcal{O}_{1:T}=1$ and $g$ satisfies
\#\label{eq_app_post_a}
\mathbb{P}(a_{1:T} | \mathcal{O}_{1:T}=1, g) &= \mathbb{P}(s_{1_T}, a_{1:T} | \mathcal{O}_{1:T}=1, g) \notag\\
&\propto \mathbb{P}( s_{1:T}, a_{1:T}, \mathcal{O}_{1:T}=1 | g)\notag\\
&= \mathbb{P}(s_1)\cdot\prod_{t=1}^T \mathbb{P}(\mathcal{O}_t = 1 | s_t, a_t, g) \cdot\mathbb{P}(a_t | s_t, g)\cdot \mathbb{P}(s_{t+1} | s_t, a_t, g)\notag\\
&\propto \prod_{t=1}^T \mathbb{P}(\mathcal{O}_t = 1 | s_t, a_t, g) \cdot\mathbb{P}(a_t | s_t, g),
\#
where the first equation and the last proportionality hold since the dynamic transition is deterministic, and the second equation holds due to Bayes' rule.

Therefore, we have
\$
\argmax_{a_{1:T}}\log\mathbb{P}(a_{1:T} | \mathcal{O}_{1:T}=1, g) &= \argmax_{a_{1:T}}\sum_{t=1}^T \log\mathbb{P}(\mathcal{O}_t = 1 | s_t, a_t, g) +\log\mathbb{P}(a_t | s_t, g),
%&=\argmax_{a_{1:T}}\sum_{t=1}^T r(s_t, a_t, g) + \lambda\mathbb{P}_{\text{LLM}}(a_t | s_t, g),
\$
where the first equation holds by taking the logarithm on the LHS and RHS of Equation \eqref{eq_app_post_a}.
\end{proof}

\subsection{Proof of Theorem \ref{thm_sample}}

\begin{proof}
With a slight abuse of notation, we denote by $\pi^*(s_{i:j})=\pi^*_i(s_{i}, g), \cdots, \pi^*_j(s_{j}, g)$ the action sequence following $\pi^*$. To show that the algorithm is optimal with probability at least $1-\delta$, it suffices to show that
\#\label{eq_app_obj}
&\mathbb{P}\biggl(\forall i\in[1, T/N],\,V_{iN+1}^\pi(s^*_{iN+1}, g) - \epsilon + \lambda\sum_{t=(i-1)N+1}^{iN} \mathbb{P}_{\text{LLM}}(a^*_t | s^*_t, g)\notag\\
&\quad\quad\quad\geq \epsilon + \lambda\max_{s_{(i-1)N+1:iN}, a_{(i-1)N+1:iN}\neq\pi^*(s_{(i-1)N+1:iN})}\sum_{t=(i-1)N+1}^{iN}\mathbb{P}_{\text{LLM}}(a_t | s_t, g) \biggr) \geq 1 - \delta,
\#
where the LHS of the inequality is the sum of the estimated value and LLM-shaped reward that corresponds to the optimal action sequence $a^*_{(i-1)N+1:iN}$, and should be greater than the RHS that corresponds to the value of any other sub-optimal action sequence with high probability. 

Then by a union bound, proving \eqref{eq_app_obj} suffices to prove that 
\#\label{eq_app_peri}
&\mathbb{P}\biggl(V_{iN+1}^\pi(s^*_{iN+1}, g) - \epsilon + \lambda\sum_{t=(i-1)N+1}^{iN} \mathbb{P}_{\text{LLM}}(a^*_t | s^*_t, g)\notag\\
&\quad\quad\quad\geq \epsilon + \lambda\max_{s_{(i-1)N+1:iN}, a_{(i-1)N+1:iN}\neq\pi^*(s_{(i-1)N+1:iN})}\sum_{t=(i-1)N+1}^{iN}\mathbb{P}_{\text{LLM}}(a_t | s_t, g) \biggr) \geq 1 - \delta/T
\#
holds for all $i\in[1, T/N]$.

Besides, we know that the $N$ random variables $\{\mathbb{P}_{\text{LLM}}(a^*_t | s^*_t, g)\}_{t=(i-1)N+1}^{iN}$ are independent and identically distributed, each following a probability density with mean $\mu$. Then according to Hoeffding's inequality, we obtain that for any constant $c>0$,
\#\label{eq_app_prob_conc}
\mathbb{P}\Biggl(\bigg|\frac{1}{N}\sum_{t=(i-1)N+1}^{iN} \mathbb{P}_{\text{LLM}}(a^*_t | s^*_t, g) - \mu\bigg| \leq c\Biggr) \geq 1 - 2\exp\Bigl(-2Nc^2\Bigr).
\#

Then with probability at least $1-2\delta / T$, 
\#\label{eq_app_dec}
\bigg|\frac{1}{N}\sum_{t=(i-1)N+1}^{iN} \mathbb{P}_{\text{LLM}}(a^*_t | s^*_t, g) - \mu\bigg| \leq \sqrt{\frac{1}{2N}\log\frac{T}{\delta}},
\#
where the inequality holds by solving the corresponding $c$ in \eqref{eq_app_prob_conc} such that the RHS is $1-2\delta / T$.

Similarly, by applying the Hoeffding's inequality, we have for any $s_t\in\mathcal{S}$ that
\$
\mathbb{P}\Bigl(\mathbb{P}_{\text{LLM}}(\pi_t^*(s_t, g) | s_t, g) \leq \mu-\sqrt{\frac{1}{2}\log(2N|\mathcal{A}|)}\Bigr) \leq \frac{1}{2N|\mathcal{A}|}.
\$

Denote the state subset that can be reached in one step at $s_{t-1}$ as $\mathcal{S}_t^{s_{t-1}}\subseteq\mathcal{S}$, where $|\mathcal{S}_t^{s_{t-1}}| \leq |\mathcal{A}|$. Then we have for all $t\in[2, T]$ and $s_{t-1}$ that
\$
\mathbb{P}\Bigl(\min_{s\in\mathcal{S}_t^{s_{t-1}}}\mathbb{P}_{\text{LLM}}(\pi_t^*(s_t, g) | s_t, g) \leq \mu-\sqrt{\frac{1}{2}\log(2N|\mathcal{A}|)}\Bigr) 
%&= \mathbb{P}\Bigl(\cup_{k}\mathcal{U}_{s_t} \leq \mu-2/3\mu\log 2kN + \sqrt{2\sigma\log 2kN}\Bigr) \\
&\leq |\mathcal{A}|\cdot\mathbb{P}\Bigl(\mathbb{P}_{\text{LLM}}(\pi^*(s) | s, g)  \leq \mu-\sqrt{\frac{1}{2}\log(2N|\mathcal{A}|)}\Bigr)\notag\\
&\leq |\mathcal{A}|\cdot \frac{1}{2N|\mathcal{A}|} = \frac{1}{2N},
\$
where the first inequality holds by applying a union bound of the $|\mathcal{A}|$ events, each of which corresponds to that the probability of the optimal action given by the LLM at a state in $\mathcal{S}_t^{s_{t-1}}$ is smaller than $\mu-\sqrt{\log(2N|\mathcal{A}|)/2}$.

Therefore, it holds for any $t\in[2, T]$ and $s_{t-1}$ that
\$
\mathbb{P}\Bigl(1- \max_{s\in\mathcal{S}_t^{s_{t-1}}, a_t\neq\pi_t^*(s_t,g)}\mathbb{P}_{\text{LLM}}(a_t | s_t, g) \leq \mu-\sqrt{\frac{1}{2}\log(2N|\mathcal{A}|)}\Bigr) \leq \frac{1}{2N}.
\$

For any state sequence $s_{(i-1)N+1:iN}$, applying the union bound over the $N$ steps, we have 
\$
&\mathbb{P}\Bigl(\exists (i-1)N+1\leq t\leq iN, \,1- \max_{s\in\mathcal{S}_t^{s_{t-1}}, a_t\neq\pi_t^*(s_t)}\mathbb{P}_{\text{LLM}}(a_t | s_t, g)\leq \mu-\sqrt{\frac{1}{2}\log(2N|\mathcal{A}|)}\Bigr)\\
&\quad\leq N\cdot \mathbb{P}\Bigl(1- \max_{s\in\mathcal{S}_t^{s_{t-1}}, a_t\neq\pi_t^*(s_t,g)}\mathbb{P}_{\text{LLM}}(a_t | s_t, g) \leq \mu-\sqrt{\frac{1}{2}\log(2N|\mathcal{A}|)}\Bigr)\leq \frac{1}{2}.
\$

Thus, we obtain
\#\label{eq_app_max}
\mathbb{P}\Bigl(\forall (i-1)N+1\leq t\leq iN, \,1- \max_{s\in\mathcal{S}_t^{s_{t-1}}, a_t\neq\pi_t^*(s_t, g)}\mathbb{P}_{\text{LLM}}(a_t | s_t, g)\geq \mu-\sqrt{\frac{1}{2}\log(2N|\mathcal{A}|)}\Bigr) \geq \frac{1}{2}.
\#

Then it holds with probability at least $1-\delta / T$ that
\$
&\sum_{t=(i-1)N+1}^{iN} \mathbb{P}_{\text{LLM}}(a^*_t | s^*_t, g) -  \max_{s_{(i-1)N+1:iN}, a_{(i-1)N+1:iN}\neq\pi^*(s_{(i-1)N+1:iN})}\sum_{t=(i-1)N+1}^{iN}\mathbb{P}_{\text{LLM}}(a_t | s_t, g)  \\
&\qquad\geq \min\Biggl\{\mu N - \sqrt{\frac{N}{2}\log\frac{T}{\delta}} + N\biggl(\mu-1-\sqrt{\frac{1}{2}\log(2N|\mathcal{A}|)}\biggr), \mu - \sqrt{\frac{1}{2}\log\frac{T}{\delta}} + \biggl(\mu-1-\sqrt{\frac{1}{2}\log(2N|\mathcal{A}|)}\biggr)\Biggr\}\\
&\qquad\geq (2\mu-1)N - \sqrt{\frac{N}{2}\log\frac{T}{\delta}} - N\sqrt{\frac{1}{2}\log(2T|\mathcal{A}|)}\\
&\qquad\geq (2\mu-1)N - N\biggl(\sqrt{\frac{1}{2}\log\frac{T}{\delta}} + \sqrt{\frac{1}{2}\log(2T|\mathcal{A}|)}\biggr),
\$
where the first inequality follows from \eqref{eq_app_dec} and \eqref{eq_app_max}.
%where the first inequality holds by basic algebra, and the second inequality holds since $\max_{a_t\in\mathcal{A}}\mathbb{P}_{\text{LLM}}(a_t | s_t, g)\geq 1/|\mathcal{A}|$ for any $s_t\in\mathcal{S}$.

Therefore, if we find the minimum $N$ that satisfies the following inequality
\#\label{eq_app_n_obj}
\min_{N\in[1, T)} V_{iN+1}^\pi(s^*_{iN+1}, g) - 2\epsilon \geq \lambda(1-2\mu) N + \lambda N\biggl(\sqrt{\frac{1}{2}\log\frac{T}{\delta}} + \sqrt{\frac{1}{2}\log(2T|\mathcal{A}|)}\biggr),
\#
then \eqref{eq_app_peri} holds for all $i\in[1, T/N]$, which further indicates \eqref{eq_app_obj}.

Solving \eqref{eq_app_n_obj} and considering the fact that exhaustive search over the $T$-horizon problem always gives the optimal solution, we obtain the stated formula of $N$.

The result is obvious since the total number of samples is $N|\mathcal{A}|^N$ in each sub-problem, and there are $T/N$ sub-problems, leading to $N|\mathcal{A}|^N\cdot T/N=T|\mathcal{A}|^N$ samples in total.
\end{proof}

\subsection{Proof of Theorem \ref{thm_sample_mc}}
\begin{proof}
By applying the Hoeffding's inequality, we obtain that
\$
\mathbb{P}\bigl(\big|\hat{V}^M_{\text{MC}}(s_t, g) - V_t^\pi(s_t, g)\big|\geq \epsilon_{\text{th}}\bigr) \leq 2\exp(-2M \epsilon_{\text{th}}^2),
\$
where the inequality holds since the expectation $\EE[\hat{V}^M_{\text{MC}}(s_t)]=V^\pi(s_t)$ and the sum of reward in one episode is in the range of $[0, 1]$. 

According to the definition of the Monte-Carlo value estimation error $\epsilon=\max_t |V_t^\pi(s_t, g) - \hat{V}^M_{\text{MC}}(s_t, g)|$, we have
\#\label{eq_mc_prob}
\mathbb{P}(e< e_{\text{th}}) \geq 1 - 2\exp(-2M \epsilon_{\text{th}}^2).
\#
Combining \eqref{eq_mc_prob} with the results in Theorem \ref{thm_sample} completes the proof.
\end{proof}
